# Supplementary material for: Multimodal Difference Learning for Sequential Recommendation
Source: arXiv:2412.08103 source file (2024-12-11)
Supplement: Supplementary file 1 [file appendix.tex]

% !TEX spellcheck = en_US
% !TeX root = main.tex

\setlength{\tabcolsep}{1.5mm}

\subsection{Supplementary parameter settings}
Our model is implemented in Pytorch\footnote{https://pytorch.org}, and our code will be made public upon acceptance.
In addition, all experiments in this paper are performed in the same experimental environment with Intel(R) Xeon(R) Silver 4210R CPU @ 2.40GHz and GeForce RTX 3090.

\begin{table}[t]
	\centering
	\setlength{\tabcolsep}{4.0mm}{
		\begin{tabular}{c|ccc}
			\hline
			\textbf{Parameters} & \textbf{ML1M} & \textbf{AKindle} & \textbf{Yelp}\\
			\hline
			\textbf{$\alpha$}            & 0.001  & 0.001  & 0.001 \\
			\textbf{$|B_u| \& |B_i|$}    & 128 & 128 & 128  \\
			\textbf{$d$}                 & 20 & 20 & 20  \\
			\hline
			\textbf{$A$}                 & 10 & 5 & 5 \\
			\textbf{$\gamma$}            & 0.01 & 0.001 & 0.1 \\
			\hline
	\end{tabular}}
	\caption{Parameter setting for three datasets.}
	\label{tab:allparamters}
\end{table}

\setlength{\tabcolsep}{1.5mm}
%\begin{table*}[htbp]
%	\centering
%	\begin{tabular}{l|cccc|cccc|cccc}
%		\hline
%		\textbf{Datasets} & \multicolumn{4}{c|}{\textbf{ML1M}} & \multicolumn{4}{c|}{\textbf{AKindle}} & \multicolumn{4}{c}{\textbf{Yelp2018}} \\
%		\hline
%		\textbf{Metrics} & \textbf{R@20} & \textbf{N@20} & \textbf{R@50} & \multicolumn{1}{c|}{\textbf{N@50}} & \textbf{R@20} & \textbf{N@20} & \textbf{R@50} & \textbf{N@50} & \textbf{R@20} & \textbf{N@20} & \textbf{R@50} & \textbf{N@50} \\
%		\hline
%		\textbf{w/o RIM} & 0.2321  & 0.3601  & 0.3900  & \multicolumn{1}{c|}{0.3774 } & 0.0803  & 0.0501  & 0.1359  & 0.0671  & 0.0611  & 0.0493  & 0.1200  & 0.0713  \\
%		\hline
%		\textbf{BiDVAE-\emph{\textbf{dCor}}} & 0.2269 & 0.3633 & 0.3938 & 0.3809 & 0.0810 & 0.0509 & 0.1374 & 0.0679 & 0.0625 & 0.0503 & 0.1219 & 0.0729 
%		\\
%		\hline
%		\textbf{BiDVAE-\emph{\textbf{CL}}} & \textbf{0.2365} & \textbf{0.3643} & \textbf{0.3944} & \textbf{0.3816} & \textbf{0.0812} & \textbf{0.0511} & \textbf{0.1378} & \textbf{0.0683} & \textbf{0.0633} & \textbf{0.0514} & \textbf{0.1227} & \textbf{0.0735} \\
%		\hline
%	\end{tabular}%
%	\caption{Performance comparisons of BiDVAE with different independence modeling manners.}
%	\label{tab:indep_manner}%
%\end{table*}%
\subsection{Data preprocessing}
The five real-world datasets used in our experiments are all from Amazon. The processing methods for datasets $\emph{Industrial and Scientific}$ and $\emph{Prime Pantry}$ differ from those for datasets $\emph{Baby}$, $\emph{Sports and Outdoors}$, and $\emph{Clothing, Shoes and Jewelry}$. In the supplementary materials, we provide different data processing codes for these two groups, which are based on MISSRec\footnote{https://github.com/gimpong/MM23-MISSRec/tree/master} and MMRec\footnote{https://github.com/enoche/MMRec}, respectively.
